# Supplementary material for: Limitations of atomistic modeling to reveal ejection of proteins from charged nanodroplets
Source: arXiv:2303.00974 source file (2023-03-02)
Supplement: Supplementary file 1 [file SI.pdf]

**Supporting Information:**

**Limitations of atomistic modeling to reveal  
ejection of proteins from charged nanodroplets**

Victor Kwan, Pranav Ballaney, Titiksha, and Styliani Consta\*

*Department of Chemistry, The University of Western Ontario, London, Ontario, Canada*

*N6A 5B7*

E-mail: [sconstas@uwo.ca](mailto:sconstas@uwo.ca)

## S1. Relaxation of myoglobin ( $1\text{MBN}^{17+}$ ) within the aqueous droplet

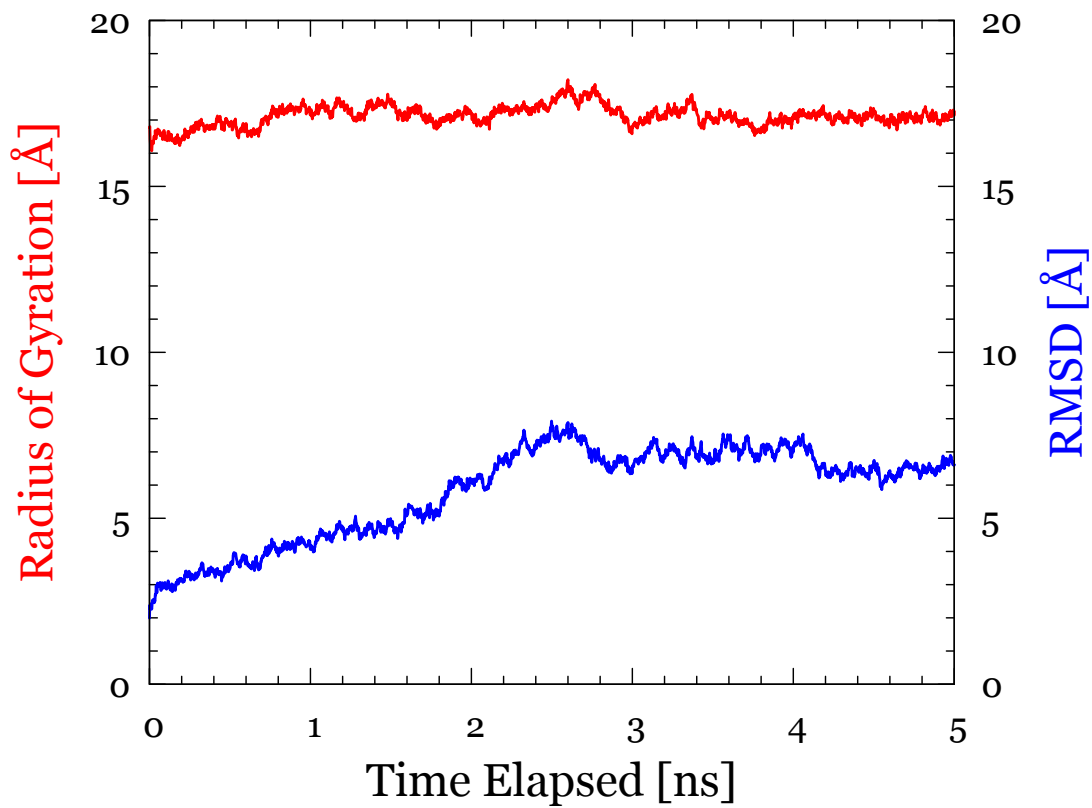

Figure S1: Radius of gyration and the root mean square deviation (RMSD) of the backbone of  $1\text{MBN}^{17+}$  restrained to the surface during equilibration.

## S2. Charging and conformations of PEG

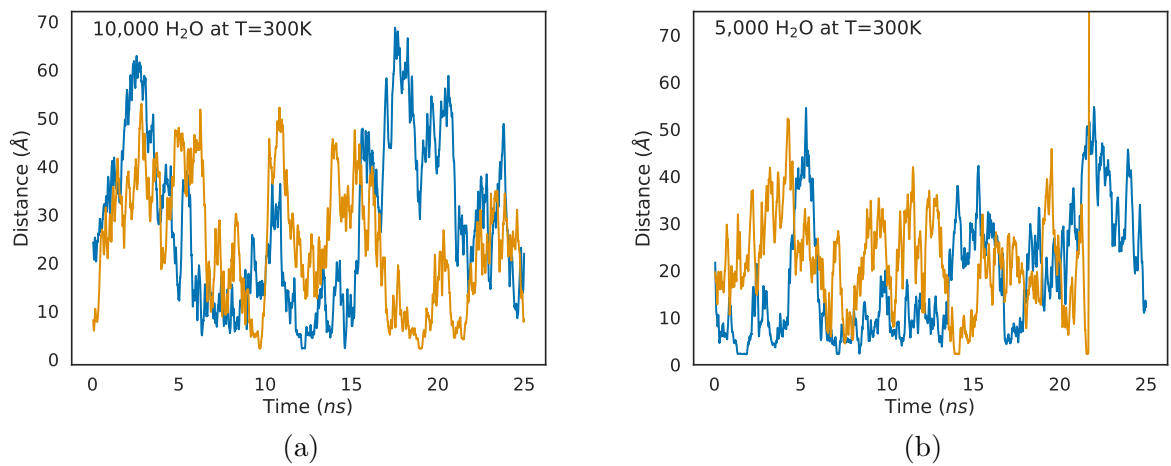

Figure S2: Same as Fig. 3 in the main text but at  $T = 300$  K.

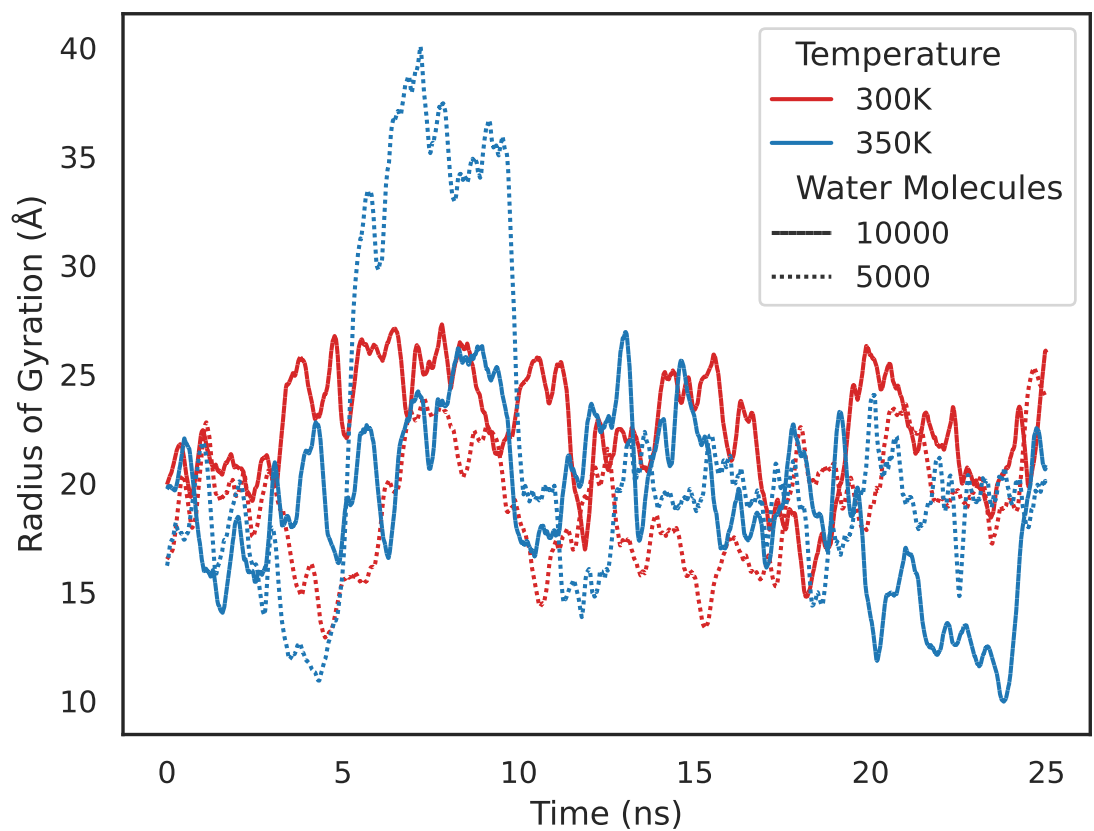

Figure S3: Time evolution of radius of gyration of PEG54.

### S3. Valine-Lysine protonated peptides

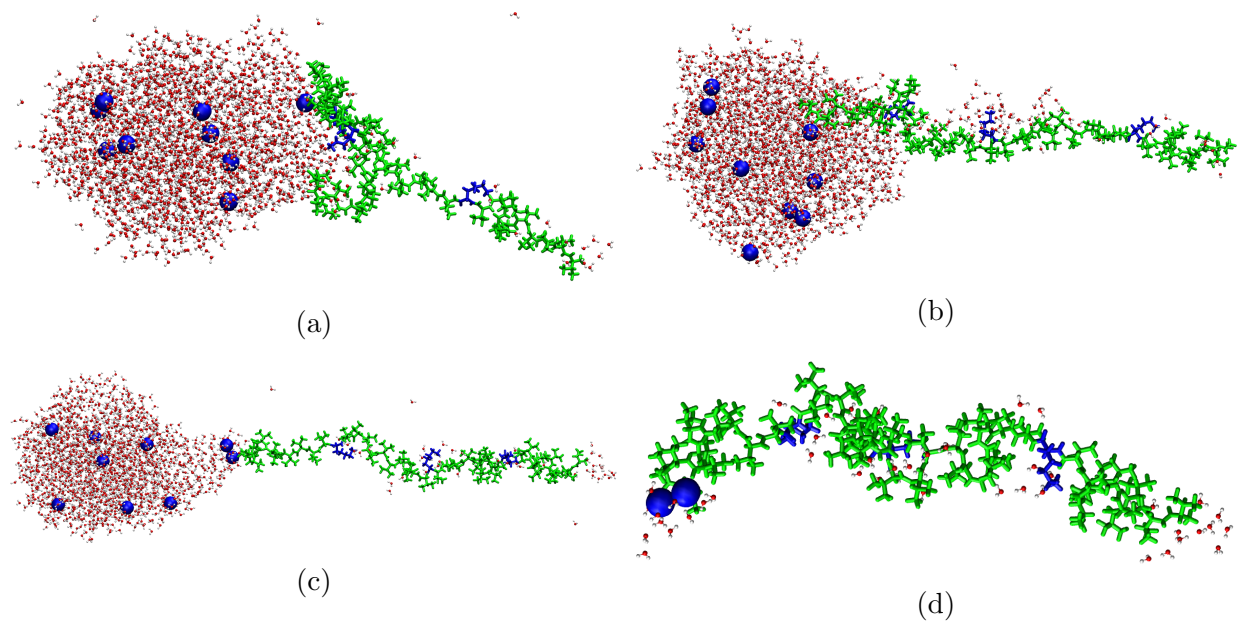

Figure S4: Snapshots of the rare event of  $[(\text{Val}_{10}-\text{Lys}^+)_3-\text{Val}_{10}]$  extrusion. The lysine and valine residues are shown in blue and green, respectively and the  $\text{Na}^+$  is shown in blue. (a) A segment of the protonated peptide extrudes. The droplet comprises 1925  $\text{H}_2\text{O}$  molecules and this extrusion occurs in 2.4 ns from the time origin (when the peptide is completely attached to the droplet). (b) The extrusion continues. The droplet comprises 1735  $\text{H}_2\text{O}$  molecules and the event occurs at 6.8 ns from the time origin. (c) The protonated peptide is completely ejected from the droplet with the assistance of two  $\text{Na}^+$  ions. The droplet comprises 1694  $\text{H}_2\text{O}$  molecules and the event occurs at 7.6 ns from the time origin. (d) The extruded peptide in gas-phase, shortly after the peptide has been totally ejected.

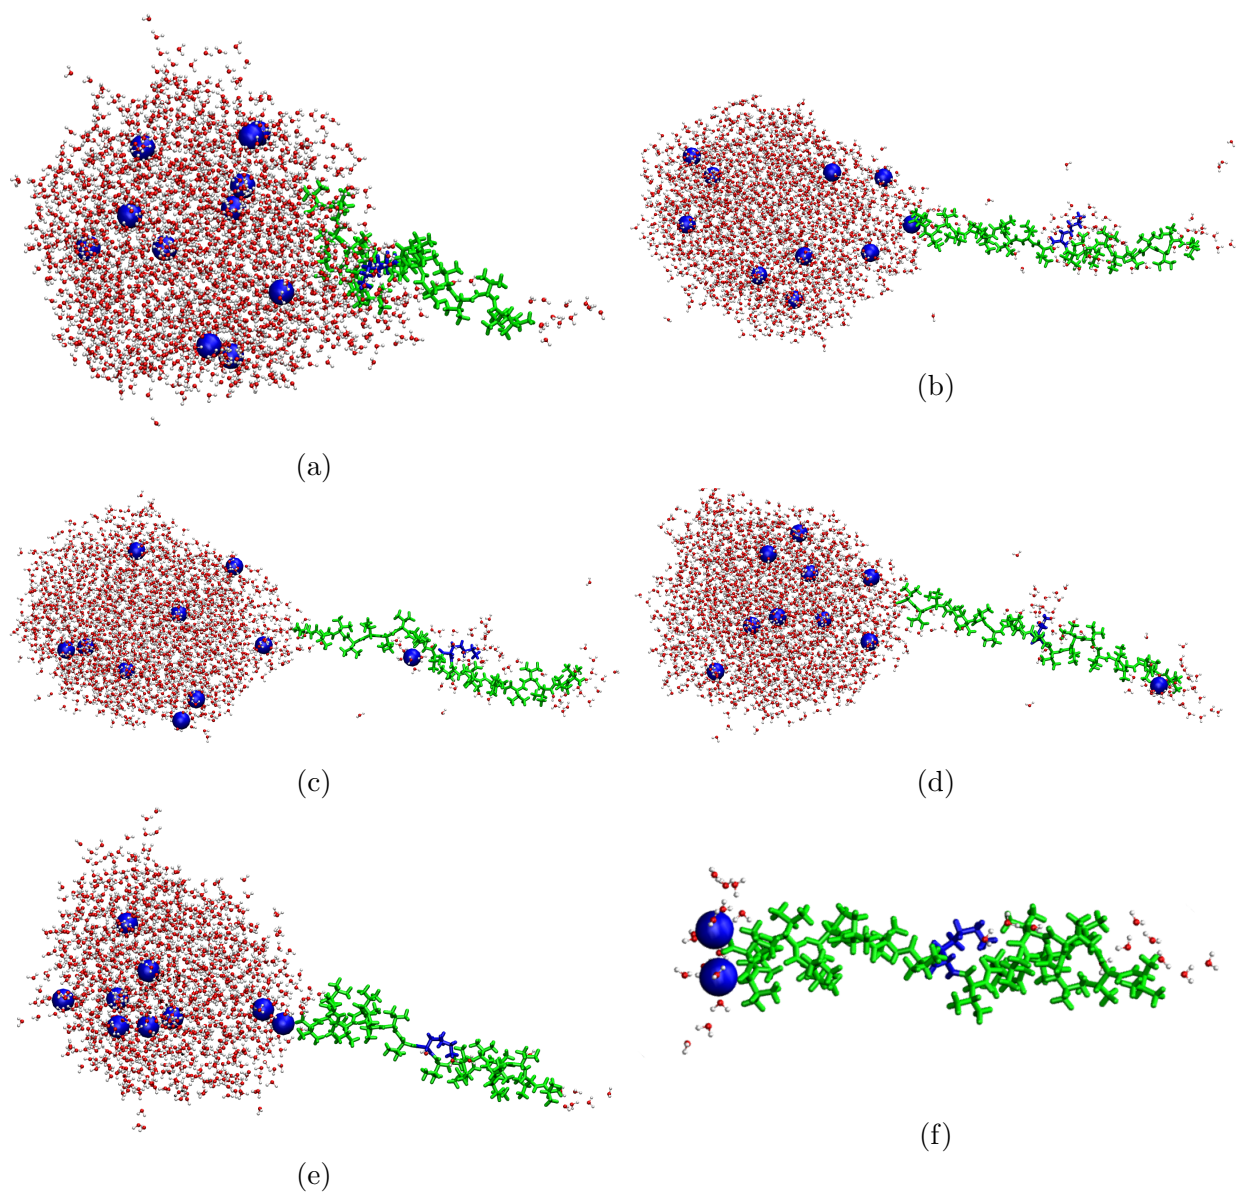

Figure S5: Snapshots of the rare event of  $[\text{Val}_{10} - \text{Lys}^+ - \text{Val}_{10}]$  ejection. The lysine and valine residues are colored blue and green, respectively, and the  $\text{Na}^+$  ions are shown in blue. (a) Extrusion of  $[\text{Val}_{10} - \text{Lys}^+ - \text{Val}_{10}]$  from a droplet comprised 1918  $\text{H}_2\text{O}$  molecules at 3.0 ns after the time origin. (b) Continuation of the extrusion, 1894  $\text{H}_2\text{O}$  molecules at 4.0 ns. (c) a  $\text{Na}^+$  travels along the peptide before being ejected from the droplet, 1880  $\text{H}_2\text{O}$  molecules at 5.0 ns. (d) A  $\text{Na}^+$  is ejected, 1872  $\text{H}_2\text{O}$  molecules at 5.4 ns. (e) The system imminently before peptide ejection, 1276  $\text{H}_2\text{O}$  molecules at 26 ns. (f) Ejected peptide.

## S4. Partial extrusion of 1WLA

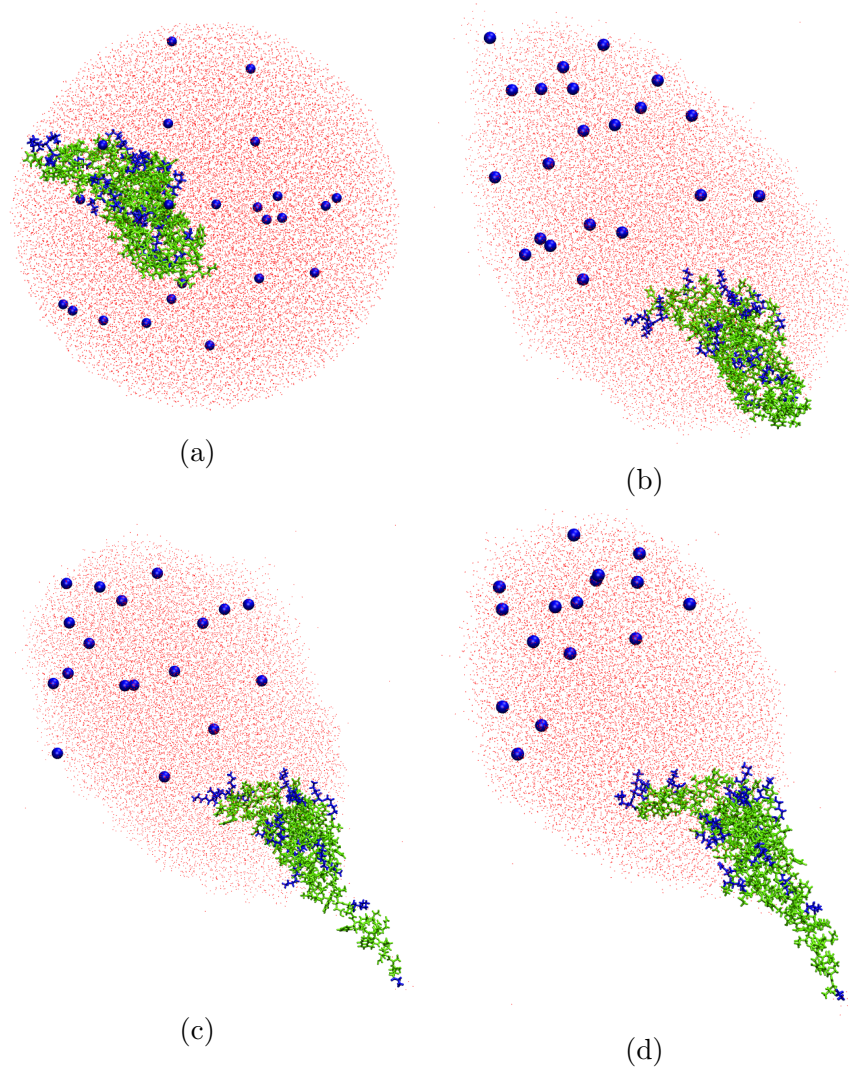

Figure S6: Snapshots of the 1WLA<sup>22+</sup>[A] partial extrusion from an aqueous droplet (see Table 2 in the main text). The charged residues are colored in blue and the uncharged residues are colored in green. Na<sup>+</sup> is shown in blue. (a) Initial configuration of the system. (b)-(d) snapshots taken every 5 ns (5 ns, 10 ns and 15 ns)

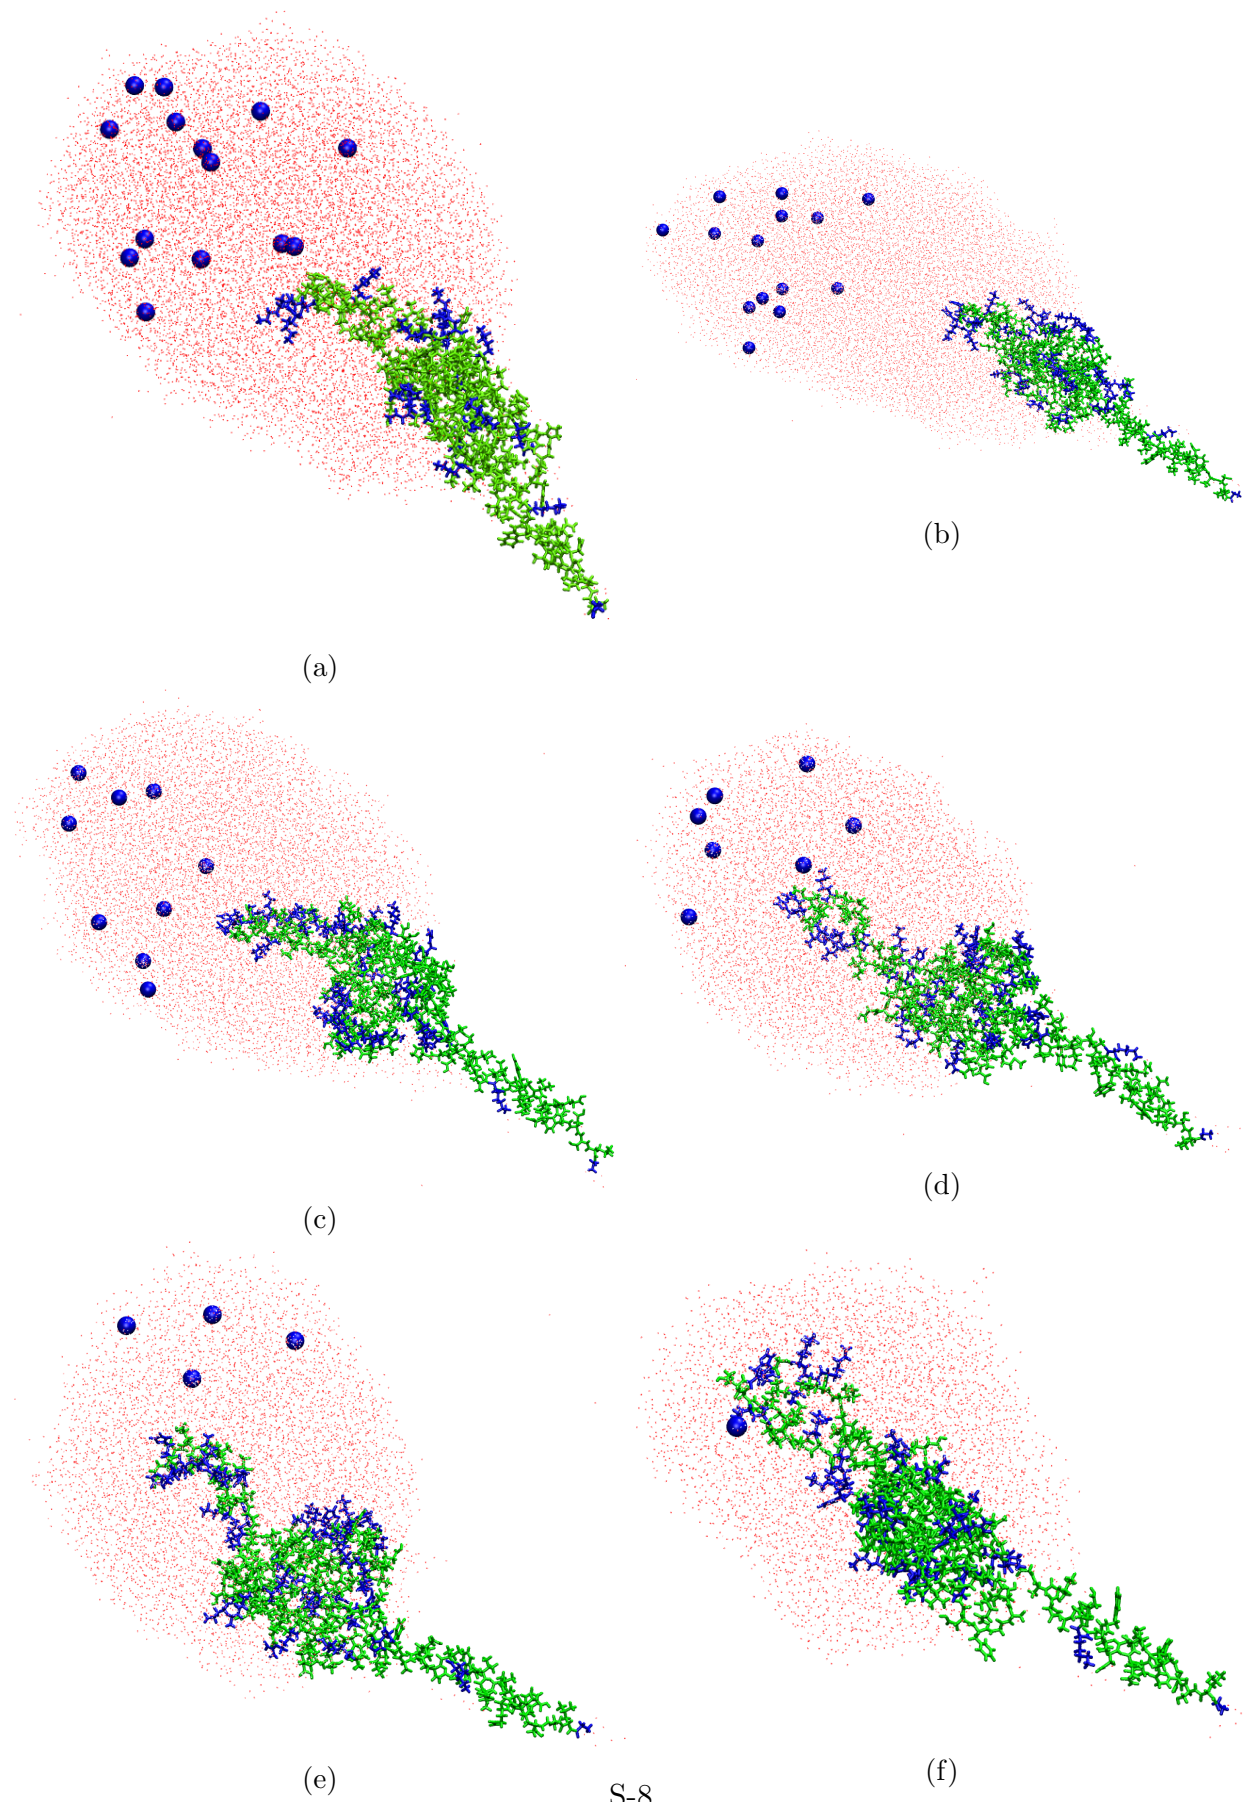

Figure S7: Continuation of Fig. S6. (a)-(f) snapshots taken every 5 ns starting from 20 ns (20 ns, 25 ns, 30 ns, 35 ns, 40 ns, 45 ns).

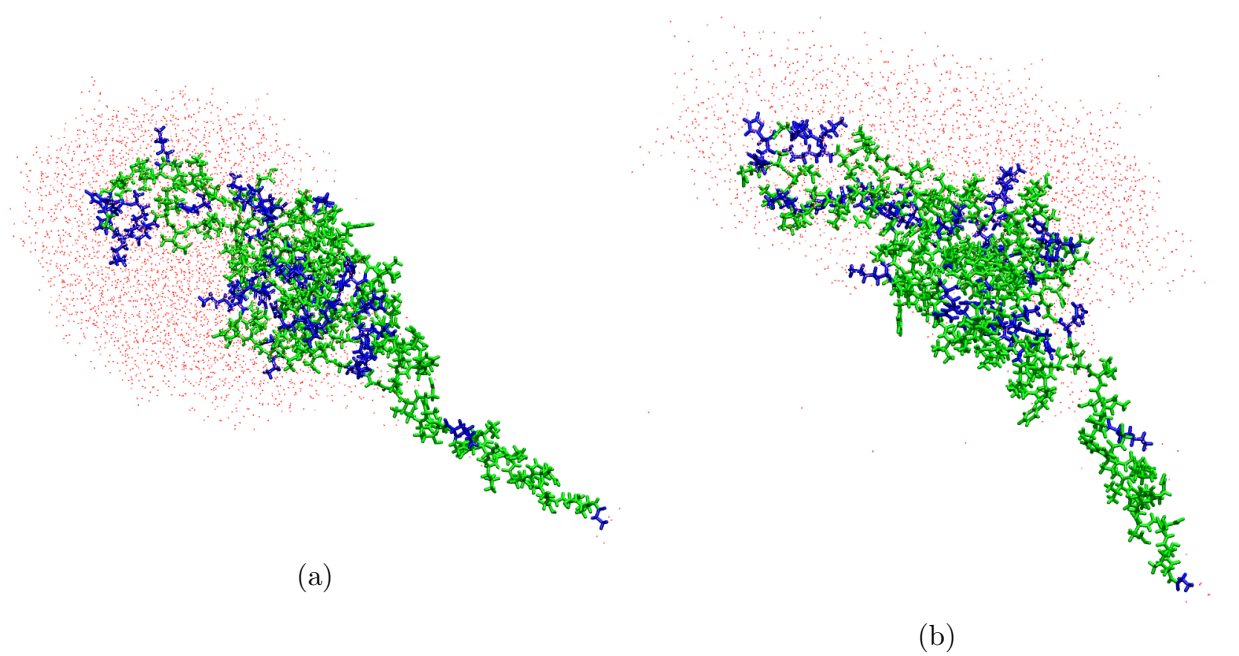

Figure S8: Continuation of Fig. S8. (a)-(b) snapshots taken every 5 ns starting from 50 ns (50 ns, 55 ns).
